# Supplementary material for: Zero-Shot Visualization: Exploring Text Corpora with User-Prompted Axes
Source: arXiv:2610.06889 source file (2026-09-23)
Supplement: Supplementary file 1 [file full-tables.tex]

This appendix reports the full mean $\pm$ SE versions of
Tables~\ref{tab:tagged_results} and \ref{tab:robustness}. Each main
table is split per dataset (one for MMLU, one for Banking77). Standard errors are computed
across MMLU subjects ($n=57$) and Banking77 intents ($n=77$).

% ============================================================
% Expansion of Table 1 (tab:tagged_results)
% ============================================================

\begin{table}[h]
\centering
\footnotesize
\setlength{\tabcolsep}{4pt}
\renewcommand{\arraystretch}{1.1}
\begin{tabular}{lccc}
\toprule
\textbf{Scorer} & \textbf{AUROC} & \textbf{AP} & \textbf{Brier}$\downarrow$ \\
\midrule
\multicolumn{4}{l}{\textit{Retriever-Based Scorers}} \\
SLR & $0.55 \pm 0.02$ & $0.07 \pm 0.01$ & $0.48 \pm \text{TBD}$ \\
DNR & $0.85 \pm 0.02$ & $0.20 \pm 0.02$ & $0.22 \pm \text{TBD}$ \\
SNR & $0.79 \pm 0.02$ & $0.17 \pm 0.02$ & $0.45 \pm \text{TBD}$ \\
\midrule
\multicolumn{4}{l}{\textit{LLM-Based Scorers}} \\
DR  & $0.86 \pm 0.01$ & $0.15 \pm 0.01$ & $0.29 \pm \text{TBD}$ \\
PZS & $0.93 \pm 0.01$ & $0.42 \pm 0.03$ & $0.14 \pm \text{TBD}$ \\
\midrule
\textit{EM-Hybrid} & $0.57 \pm 0.02$ & $0.11 \pm 0.02$ & $0.44 \pm \text{TBD}$ \\
\bottomrule
\end{tabular}
\caption{MMLU. Full mean $\pm$ SE for Table~\ref{tab:tagged_results}.}
\label{tab:tagged_mmlu_full}
\end{table}

\begin{table}[h]
\centering
\footnotesize
\setlength{\tabcolsep}{4pt}
\renewcommand{\arraystretch}{1.1}
\begin{tabular}{lccc}
\toprule
\textbf{Scorer} & \textbf{AUROC} & \textbf{AP} & \textbf{Brier}$\downarrow$ \\
\midrule
\multicolumn{4}{l}{\textit{Retriever-Based Scorers}} \\
SLR & $0.84 \pm 0.01$ & $0.30 \pm 0.02$ & $0.35 \pm \text{TBD}$ \\
DNR & $0.95 \pm 0.01$ & $0.55 \pm 0.03$ & $0.21 \pm \text{TBD}$ \\
SNR & $0.94 \pm 0.01$ & $0.54 \pm 0.03$ & $0.20 \pm \text{TBD}$ \\
\midrule
\multicolumn{4}{l}{\textit{LLM-Based Scorers}} \\
DR  & $0.69 \pm 0.02$ & $0.06 \pm 0.01$ & $0.36 \pm \text{TBD}$ \\
PZS & $0.95 \pm 0.01$ & $0.55 \pm 0.03$ & $0.11 \pm \text{TBD}$ \\
\midrule
\textit{EM-Hybrid} & $0.84 \pm 0.01$ & $0.42 \pm 0.03$ & $0.27 \pm \text{TBD}$ \\
\bottomrule
\end{tabular}
\caption{Banking77. Full mean $\pm$ SE for Table~\ref{tab:tagged_results}.}
\label{tab:tagged_banking_full}
\end{table}

% ============================================================
% Expansion of Table 2 (tab:robustness)
% ============================================================

\begin{table}[h]
\centering
\footnotesize
\setlength{\tabcolsep}{4pt}
\renewcommand{\arraystretch}{1.1}
\begin{tabular}{lccc}
\toprule
\textbf{Model} & \textbf{AUROC} & \textbf{AP} & \textbf{Brier}$\downarrow$ \\
\midrule
Qwen-3B    & $0.93 \pm 0.01$ & $0.42 \pm 0.03$ & $0.40 \pm \text{TBD}$ \\
Mistral-7B & $0.93 \pm 0.01$ & $0.42 \pm 0.03$ & $0.14 \pm \text{TBD}$ \\
Llama-8B   & $0.94 \pm 0.01$ & $0.42 \pm 0.03$ & $0.22 \pm \text{TBD}$ \\
Gemma-9B   & $0.96 \pm 0.01$ & $0.50 \pm 0.04$ & $0.10 \pm \text{TBD}$ \\
\bottomrule
\end{tabular}
\caption{MMLU. Full mean $\pm$ SE for Table~\ref{tab:robustness}.}
\label{tab:robustness_mmlu_full}
\end{table}

\begin{table}[h]
\centering
\footnotesize
\setlength{\tabcolsep}{4pt}
\renewcommand{\arraystretch}{1.1}
\begin{tabular}{lccc}
\toprule
\textbf{Model} & \textbf{AUROC} & \textbf{AP} & \textbf{Brier}$\downarrow$ \\
\midrule
Qwen-3B    & $0.94 \pm 0.01$ & $0.52 \pm 0.03$ & $0.28 \pm \text{TBD}$ \\
Mistral-7B & $0.95 \pm 0.01$ & $0.55 \pm 0.03$ & $0.11 \pm \text{TBD}$ \\
Llama-8B   & $0.92 \pm 0.01$ & $0.45 \pm 0.03$ & $0.22 \pm \text{TBD}$ \\
Gemma-9B   & $0.96 \pm 0.01$ & $0.63 \pm 0.03$ & $0.09 \pm \text{TBD}$ \\
\bottomrule
\end{tabular}
\caption{Banking77. Full mean $\pm$ SE for Table~\ref{tab:robustness}.}
\label{tab:robustness_banking_full}
\end{table}
